# Supplementary material for: Myopic Bayesian Design of Experiments via Posterior Sampling and Probabilistic Programming
Source: arXiv:1805.09964 source file (2018-05-25)
Supplement: Supplementary file 1 [file coxSupp.pdf]

## A Some Ancillary Material

We will need the following technical results for our analysis. The first is a version of Pinsker's inequality.

**Lemma 4** (Pinsker's inequality). *Let  $X, Z \in \mathcal{X}$  be random quantities and  $f : \mathcal{X} \rightarrow [0, B]$ . Then,*  

$$|\mathbb{E}[f(X)] - \mathbb{E}[f(Z)]| \leq B\sqrt{\frac{1}{2}\text{KL}(P(X)\|P(Z))}.$$

The next, taken from Russo and Van Roy [43], relates the KL divergence to the mutual information for two random quantities  $X, Y$ .

**Lemma 5** (Russo and Van Roy [43], Fact 6). *For random quantities  $X, Z \in \mathcal{X}$ ,*  

$$I(X; Z) = \mathbb{E}_X[\text{KL}(P(Y|X)\|P(Y))].$$

**Lemma 6.** *Let  $X, Y, Z$  be random quantities such that  $Y$  is a deterministic function of  $X$ . Then,*  

$$I(Y; Z) \leq I(X; Z).$$

*Proof.* Let  $Y'$  capture the remaining randomness in  $X$  so that  $X = Y \cup Y'$ . Then, since conditioning reduces entropy,  $I(Y; Z) = H(Z) - H(Z|Y) \leq H(Z) - H(Z|Y \cup Y') = I(X; Z)$ .  $\square$

## B Proofs

### B.1 Notation and Set up

In this subsection, we will introduce some notation, prove some basic lemmas, and in general, lay the groundwork for our analysis.  $\mathbb{P}, \mathbb{E}$  denote probabilities and expectations.  $\mathbb{P}_t, \mathbb{E}_t$  denote probabilities and expectations when conditioned on the actions and observations up to and including time  $t$ , e.g. for any event  $E$ ,  $\mathbb{P}_t(E) = \mathbb{P}(E|D_t)$ . For two data sequences  $A, B$ ,  $A \uplus B$  denotes the concatenation of the two sequences. When  $x \in \mathcal{X}$ ,  $Y_x$  will denote the random observation from  $\mathbb{P}(Y|x, \theta)$ .

Let  $D_t \in \mathcal{D}_t$  be a data sequence of length  $t$ . Then,  $Q^\pi(D_t, x, y)$  will denote the expected total penalty when we take action  $x \in \mathcal{X}$ , observe  $y \in \mathcal{Y}$  and then execute policy  $\pi$  for the remaining  $n - t - 1$  steps. That is,

$$\begin{aligned} Q^\pi(D_t, x, y) &= \mathbb{E}[\Lambda(\theta_\star, D_t \uplus \{(x, y)\} \uplus F_{t+2:n})] \\ &= \sum_{j=1}^t \lambda(\theta_\star, D_j) + \lambda(\theta_\star, D_j \uplus \{(x, y)\}) + \mathbb{E}_{F_{t+2:n}} \left[ \sum_{j=t+2}^n \lambda(\theta_\star, D_j \uplus \{(x, y)\} \uplus F_{t+2:j}) \right]. \end{aligned} \quad (4)$$

Here, the action-observation pairs collected by  $\pi$  from steps  $t + 2$  to  $n$  are  $F_{t+2:n}$ . The expectation is over the observations and any randomness in  $\pi$ . While we have omitted for conciseness,  $Q^\pi$  is a function of the true parameter  $\theta_\star$ . Let  $d_\pi^t$  denote the distribution of  $D_t$  when following a policy  $\pi$  for the first  $t$  steps. We then have,

$$J(\theta_\star, \pi) = \mathbb{E}_{D_t \sim d_\pi^t} [\mathbb{E}_{X \sim \pi(D_t)} [Q^\pi(D_t, X, Y)]], \quad (5)$$

where, recall,  $Y_X$  is drawn from  $\mathbb{P}(Y|X, \theta_\star)$ . The following Lemma decomposes the regret  $J_n(\theta_\star, \pi) - J_n(\theta_\star, \pi_M^\star)$  as a sum of terms which are convenient to analyse. The proof is adapted from Lemma 4.3 in Ross and Bagnell [41].

**Lemma 7.** *For any two policies  $\pi_1, \pi_2$ ,*

$$\begin{aligned} J(\theta_\star, \pi_1) - J(\theta_\star, \pi_2) &= \\ &= \sum_{t=1}^n \mathbb{E}_{D_{t-1} \sim d_{\pi_1}^{t-1}} [\mathbb{E}_{X \sim \pi_1(D_{t-1})} [Q^{\pi_2}(D_{t-1}, X, Y_X)] - \mathbb{E}_{X \sim \pi_2(D_{t-1})} [Q^{\pi_2}(D_{t-1}, X, Y_X)]] \end{aligned}$$

479 *Proof.* Let  $\pi^t$  be the policy that follows  $\pi_1$  from time step 1 to  $t$ , and then executes policy  $\pi_2$  from  
 480  $t + 1$  to  $n$ . Hence, by (5),

$$\begin{aligned} J(\theta_*, \pi^t) &= \mathbb{E}_{D_{t-1} \sim d_{\pi_1}^{t-1}} [\mathbb{E}_{X \sim \pi_1(D_{t-1})} [Q^{\pi_2}(D_{t-1}, X, Y_X)]] \\ &= \mathbb{E}_{D_t \sim d_{\pi_1}^t} [\mathbb{E}_{X \sim \pi_2(D_t)} [Q^{\pi_2}(D_t, X, Y_X)]] . \end{aligned}$$

481 The claim follows from the observation,  $J(\theta_*, \pi_1) - J(\theta_*, \pi_2) = J(\theta_*, \pi^n) - J(\theta_*, \pi^0) =$   
 482  $\sum_{t=1}^n J(\theta_*, \pi^t) - J(\theta_*, \pi^{t-1})$ .  $\square$

483 We will use Lemma 7 with  $\pi_2$  as the policy  $\pi_M^*$  which knows  $\theta_*$  and with  $\pi_1$  as the policy  $\pi$  whose  
 484 regret we wish to bound. For this, denote the action chosen by  $\pi$  when it has seen data  $D_{t-1}$  as  $X_t$   
 485 and that taken by  $\pi_M^*$  as  $X'_t$ . By Lemma 7 and equation (4) we have,

$$\mathbb{E}_{\theta_*} [J(\theta_*, \pi) - J(\theta_*, \pi_M^*)] = \sum_{t=1}^n \mathbb{E}_{t-1} [Q^{\pi_M^*}(D_{t-1}, X_t, Y_{X_t}) - Q^{\pi_M^*}(D_{t-1}, X'_t, Y_{X'_t})] .$$

486 Note that  $\mathbb{E}_{t-1}$ , which conditions on the data sequence  $D_{t-1}$  collected by  $\pi$ , encompasses three  
 487 sources of randomness. The first is due to the randomness in the problem due to  $\theta_* \sim \rho_0$ , the second  
 488 is due to the observations  $Y \sim \mathbb{P}(\cdot | X, \theta_*)$ , and the third is an external source of randomness  $U$  used  
 489 by the decision maker in step 3 in Algorithm 1. While the actions  $\{X_t\}_t$  chosen depends on all  
 490 sources of randomness, these three sources are themselves independent. For example, we can write  
 491  $\mathbb{E}_{t-1}[\cdot] = \mathbb{E}_U[\mathbb{E}_{t-1, \rho}[\mathbb{E}_{t-1, Y}[\cdot]]]$  where  $\mathbb{E}_U$  captures the randomness by the decision maker,  $\mathbb{E}_{t-1, \rho}$   
 492 due to the prior and  $\mathbb{E}_{t-1, Y}$  due to the observations. With this in consideration, define

$$q_t(x, y) = \mathbb{E}_{Y_{t+1:n}} [Q^{\pi_M^*}(D_{t-1}, x, y)] , \quad (6)$$

493 where  $\mathbb{E}_{Y_{t+1:n}}$  is the expectation over the observations from time step  $t + 1$  to  $n$ .  $q_t$  is the expected  
 494 total penalty when we have data  $D_{t-1}$  collected by  $\pi$ , then execute action  $x$  at time  $t$ , observe  $y$  and  
 495 then follow  $\pi_M^*$  for the remaining time steps. Note that  $q_t$  is a deterministic function of  $\theta_*$ ,  $x$ , and  $y$   
 496 since  $\pi_M^*$  is a deterministic policy and the randomness of future observations has been integrated out.  
 497 We can now write,

$$\mathbb{E}[J(\theta_*, \pi) - J(\theta_*, \pi_M^*)] = \sum_{t=1}^n \mathbb{E}_{t-1} [q_t(X_t, Y_{X_t}) - q_t(X'_t, Y_{X'_t})] , \quad (7)$$

498 where  $\mathbb{E}_{t-1}$  inside the summation is over the randomness in  $\theta_*$ , the randomness of the policy in  
 499 choosing  $X_t$  and the observations  $Y_{X_t}, Y_{X'_t}$ .

## 500 B.2 Proof of Theorem 2

501 We will let  $\tilde{\mathbb{P}}_{t-1}$  denote the distribution of  $X_t$  given  $D_{t-1}$ ; i.e.  $\tilde{\mathbb{P}}_{t-1}(\cdot) = \mathbb{P}_{t-1}(X_t = \cdot)$ . The density  
 502 (Radon-Nikodym derivative)  $\tilde{p}_{t-1}$  of  $\tilde{\mathbb{P}}_{t-1}$  can be expressed as  $\tilde{p}_{t-1}(x) = \int_{\Theta} p_*(x|\theta) p(\theta|D_{t-1}) d\theta$   
 503 where  $p_*(x|\theta)$  is the density of the maximiser given  $\theta$  and  $p(\theta|D_{t-1})$  is the posterior density of  $\theta$   
 504 conditioned on  $D_{t-1}$ . Hence,  $X_t$  has the same distribution as  $X'_t$ ; i.e.  $\mathbb{P}_{t-1}(X'_t = \cdot) = \tilde{\mathbb{P}}_{t-1}(\cdot)$ . This  
 505 will form a key intuition in our analysis. To this end, we begin with a technical result, whose proof  
 506 is adapted from Russo and Van Roy [43]. We will denote by  $I_{t-1}(A; B)$  the mutual information  
 507 between two variables  $A, B$  under the posterior measure after having seen  $D_{t-1}$ ; i.e.  $I_{t-1}(A; B) =$   
 508  $\text{KL}(\mathbb{P}_{t-1}(A, B) \| \mathbb{P}_{t-1}(A) \cdot \mathbb{P}_{t-1}(B))$ .

509 **Lemma 8.** Assume that we have collected a data sequence  $D_{t-1}$ . Let the action taken by  $\pi_M^{\text{PS}}$  at  
 510 time instant  $t$  with  $D_{t-1}$  be  $X_t$  and the action taken by  $\pi_M^*$  be  $X'_t$ . Then,

$$\begin{aligned} \mathbb{E}_{t-1}[q_t(X_t, Y_{X_t}) - q_t(X'_t, Y_{X'_t})] &= \sum_{x \in \mathcal{X}} (\mathbb{E}_{t-1}[q_t(x, Y_x)] - \mathbb{E}_{t-1}[q_t(x, Y_x) | X'_t = x]) \tilde{\mathbb{P}}_{t-1}(x) \\ I_{t-1}(X'_t; (X_t, Y_{X_t})) &= \sum_{x_1, x_2 \in \mathcal{X}} \text{KL}(\mathbb{P}_{t-1}(Y_{x_1} | X'_t = x_2) \| \mathbb{P}_{t-1}(Y_{x_1})) \tilde{\mathbb{P}}_{t-1}(x_1) \tilde{\mathbb{P}}_{t-1}(x_2) \end{aligned}$$

511 *Proof.* The proof for both results uses the fact that  $\mathbb{P}_{t-1}(X_t = x) = \mathbb{P}_{t-1}(X'_t = x) = \tilde{\mathbb{P}}_{t-1}(x)$ . For  
 512 the first result,

$$\begin{aligned}
 & \mathbb{E}_{t-1}[q_t(X_t, Y_{X_t}) - q_t(X'_t, Y_{X'_t})] \\
 &= \sum_{x \in \mathcal{X}} \mathbb{P}_{t-1}(X_t = x) \mathbb{E}_{t-1}[q_t(X_t, Y_{X_t}) | X_t = x] - \sum_{x \in \mathcal{X}} \mathbb{P}_{t-1}(X'_t = x) \mathbb{E}_{t-1}[q_t(X'_t, Y_{X'_t}) | X'_t = x] \\
 &= \sum_{x \in \mathcal{X}} \mathbb{P}_{t-1}(X_t = x) \mathbb{E}_{t-1}[q_t(x, Y_x)] - \sum_{x \in \mathcal{X}} d\mathbb{P}_{t-1}(X'_t = x) \mathbb{E}_{t-1}[q_t(x, Y_x) | X'_t = x] \\
 &= \sum_{x \in \mathcal{X}} (\mathbb{E}_{t-1}[q_t(x, Y_x)] - \mathbb{E}_{t-1}[q_t(x, Y_x) | X'_t = x]) \tilde{\mathbb{P}}_{t-1}(x).
 \end{aligned}$$

513 The second step uses the fact that the observation  $Y_x$  does not depend on the fact that  $x$  may have been  
 514 chosen by  $\pi_M^{\text{PS}}$ ; this is because  $\pi_M^{\text{PS}}$  makes its decisions based on past data  $D_{t-1}$  and is independent  
 515 of  $\theta_*$  given  $D_{t-1}$ .  $Y_x$  however can depend on the fact that  $x$  may have been the action chosen by  $\pi_M^*$   
 516 which knows  $\theta_*$ . For the second result,

$$\begin{aligned}
 & \mathbb{I}_{t-1}(X'_t; (X_t, Y_{X_t})) = \mathbb{I}_{t-1}(X'_t; X_t) + \mathbb{I}_{t-1}(X'_t; Y_{X_t} | X_t) = \mathbb{I}_{t-1}(X'_t; Y_{X_t} | X_t) \\
 &= \sum_{x_1 \in \mathcal{X}} \mathbb{P}_{t-1}(X_t = x_1) \mathbb{I}_{t-1}(X'_t; Y_{X_t} | X_t = x) = \sum_{x_1 \in \mathcal{X}} \tilde{\mathbb{P}}_{t-1}(x_1) d(x) \mathbb{I}_{t-1}(X'_t; Y_{x_1}) \\
 &= \sum_{x_1 \in \mathcal{X}} \tilde{\mathbb{P}}_{t-1}(x_1) d(x) \sum_{x_2 \in \mathcal{X}} \mathbb{P}_{t-1}(X'_t = x_2) \text{KL}(\mathbb{P}(Y_{x_1} | X'_t = x_2) \| \mathbb{P}(Y_{x_1})) \\
 &= \sum_{x_1, x_2 \in \mathcal{X}} \text{KL}(\mathbb{P}_{t-1}(Y_{x_1} | X'_t = x_2) \| \mathbb{P}_{t-1}(Y_{x_1})) \tilde{p}_{t-1}(x_1) \tilde{p}_{t-1}(x_2)
 \end{aligned}$$

517 The first step uses the chain rule for mutual information. The second step uses that  $X_t$  is chosen  
 518 based on an external source of randomness and  $D_{t-1}$ ; therefore, it is independent of  $\theta_*$  and hence  
 519  $X'_t$  given  $D_{t-1}$ . The fourth step uses that  $Y_{x_1}$  is independent of  $X_t$ . The fifth step uses lemma 5 in  
 520 Appendix A.  $\square$

521 The next Lemma uses the conditions on  $\lambda$  given in Section 4 to show that  $q_t$  (6) is bounded. This  
 522 essentially establishes that the effect of a single bad action is bounded on the long run penalties.

523 **Lemma 9.** Let  $B$  be as given in Theorem 2 for any of conditions 1.1-1.3. Then,  $\sup q_t - \inf q_t \leq B$ .

524 *Proof.* In this proof,  $(x, y), (x', y') \in \mathcal{X} \times \mathcal{Y}$  will be two pairs of action-observations. Denote the  
 525 action-observations pairs when following  $\pi_M^*$  after  $(x, y)$  by  $H_{t:n}$ , i.e.  $H_{t:n}$  starts with  $(x, y)$  and has  
 526 length  $n - t + 1$ . Similarly define  $H'_{t:n}$  for  $(x', y')$ . Then  $q_t(x, y) - q_t(x', y') = \mathbb{E}_{Y_{t+1:n}}[r_t]$ , where,

$$\begin{aligned}
 r_t &= \Lambda(\theta_*, D_{t-1} \uplus H_{t:n}) - \Lambda(\theta_*, D_{t-1} \uplus H'_{t:n}) \\
 &= \sum_{j=t}^n \left( \lambda(\theta_*, D_{t-1} \uplus H_{t:j}) - \lambda(\theta_*, D_{t-1} \uplus H'_{t:j}) \right) \tag{8}
 \end{aligned}$$

527 We will now prove  $q_t(x, y) - q_t(x', y') \leq B$  separately for each condition.

528 **Condition 1.1:** Under this setting,  $\pi_M^*$  which knows  $\theta_*$ , will behave identically after the end of the  
 529 current episode. This is because the penalty at the next episode will not depend on the data collected  
 530 during the current episode. Therefore, the summation in (8) is from  $t$  to the end of the episode  $s$ . We  
 531 hence have,  $r_t \leq s - t \leq H = B$ .

532 **Condition 1.2:** Denote  $\epsilon_j = \lambda(\theta_*, D_{t-1} \uplus H_{t:j}) - \lambda(\theta_*, D_{t-1} \uplus H'_{t:j})$ .  $\epsilon_j$  is a random quantity for  
 533  $j \geq t + 1$  as it depends on the observations. We have  $r_t = \sum_{j=t}^n \epsilon_j$ . Observe that, at time step  $j$ ,  $\pi_M^*$   
 534 chooses the action to maximise  $\mathbb{E}_{Y_x}[\lambda(\theta_*, D_{t-1} \uplus H_{t:j} \uplus \{(x, Y_x)\})]$  when starting with  $(x, y)$ , and  
 535  $\mathbb{E}_{Y_{x'}}[\lambda(\theta_*, D_{t-1} \uplus H'_{t:j} \uplus \{(x', Y_{x'})\})]$  when starting with  $(x', y')$ . Hence, condition 1.2 implies that,  
 536  $\mathbb{E}_{Y_{j+1}}[\epsilon_{j+1}] \leq \alpha \epsilon_j$ . An inductive argument leads us to,  $\mathbb{E}_{Y_{t+1}, \dots, Y_j}[\epsilon_j] \leq \alpha^{j-t} \epsilon_t$ . However, since  $\lambda$   
 537 maps to  $[0, 1]$ ,  $\epsilon_t \leq 1$ . Hence  $\mathbb{E}_{Y_{t+1:n}}[r_t] \leq \sum_j \alpha^{j-t} \epsilon_t \leq 1/(1 - \alpha) = B$ .

538 **Condition 1.3:** For the purposes of this analysis, we will allow a decision maker to take no action at  
 539 time  $t - 1$  and denote this by  $\emptyset$ , i.e.  $D_{t-1} \uplus \emptyset \uplus F_{t+1:n}$  means the action observation pairs were

540  $D_{t-1}$  from time 1 to  $t-1$ , then there was no action at time  $t$  and then from time  $t+1$  to  $n$ , the action  
 541 observation pairs were  $F_{t+1:n}$ . In doing so, the decision maker incurs a penalty of  $\lambda(\theta_*, D_{t-1})$  at  
 542 step  $t+1$ . Correspondingly, we have,

$$\Lambda(\theta_*, D_{t-1} \uplus \emptyset \uplus F_{t+2:n}) = \sum_{j=1}^{t-1} \lambda(\theta_*, D_j) + \lambda(\theta_*, D_{t-1}) + \sum_{j=t+2}^n \lambda(\theta_*, D_{t-1} \uplus F_{t+1:j}).$$

543 Adding and subtracting  $\Lambda(\theta_*, D_{t-1} \uplus \emptyset \uplus H'_{t+1:n-1})$  to  $r_t$  we have,

$$\begin{aligned} r_t &= (\Lambda(\theta_*, D_{t-1} \uplus H_{t:n}) - \Lambda(\theta_*, D_{t-1} \uplus \emptyset \uplus H'_{t+1:n-1})) + \\ &\quad (\Lambda(\theta_*, D_{t-1} \uplus \emptyset \uplus H'_{t+1:n-1}) - \Lambda(\theta_*, D_{t-1} \uplus H'_{t:n})). \end{aligned} \quad (9)$$

544 The second term above can be bounded by 1 since  $\lambda$  maps to  $[0, 1]$ .

$$\begin{aligned} &\Lambda(\theta_*, D_{t-1} \uplus \emptyset \uplus H'_{t+1:n-1}) - \Lambda(\theta_*, D_{t-1} \uplus H'_{t:n}) \\ &= \lambda(\theta_*, D_{t-1}) + \sum_{j=t+1}^{n-1} \lambda(\theta_*, D_{t-1} \uplus H'_{t:j}) - \sum_{j=t+1}^n \lambda(\theta_*, D_{t-1} \uplus H'_{t:j}) \\ &= \lambda(\theta_*, D_{t-1}) - \lambda(\theta_*, D_{t-1} \uplus H'_{t:n}) \leq 1. \end{aligned} \quad (10)$$

545 For the first term, we have,

$$\begin{aligned} &(\Lambda(\theta_*, D_{t-1} \uplus H_{t:n}) - \Lambda(D_{t-1} \uplus \emptyset \uplus H'_{t+1:n-1})) \\ &= (\lambda(\theta_*, D_{t-1} \uplus \{(x, y)\}) - \lambda(\theta_*, D_{t-1})) + \sum_{j=t+1}^n (\lambda(\theta_*, D_t \uplus H_{t:j}) - \lambda(\theta_*, D_t \uplus H'_{t:j-1})). \end{aligned} \quad (11)$$

546 Recall that the actions in  $H_{t:j}$  are chosen to maximise the expected future rewards. By condition 1.3  
 547 and since  $D_{t-1} \cup \{(x, y)\} \supset D_{t-1}$ , each of the  $n-t$  terms in the RHS summation is less than or  
 548 equal to zero in expectation over the observations. Since  $\lambda(\theta_*, D_{t-1} \uplus \{(x, y)\}) - \lambda(\theta_*, D_{t-1}) \leq 1$ ,  
 549 the above term is at most 1 in expectation over  $\mathbb{E}_{Y,t+1:n}$ . Combining this with (10) gives us  
 550  $\mathbb{E}_{Y,t+1:n}[r_t] \leq 2 = B$ .  $\square$

551 We are now ready to prove theorem 2.

552 **Proof of Theorem 2:** Using the first result of Lemma 8, we have,

$$\begin{aligned} &\mathbb{E}_{t-1}[q_t(X_t, Y_{X_t}) - q_t(X'_t, Y_{X'_t})]^2 \\ &= \left( \sum_{x \in \mathcal{X}} \tilde{\mathbb{P}}_{t-1}(x) (\mathbb{E}_{t-1}[q_t(x, Y_x)] - \mathbb{E}_{t-1}[q_t(x, Y_x) | X'_t = x]) \right)^2 \\ &\leq |\mathcal{X}| \sum_{x \in \mathcal{X}} \tilde{\mathbb{P}}_{t-1}(x)^2 (\mathbb{E}_{t-1}[q_t(x, Y_x)] - \mathbb{E}_{t-1}[q_t(x, Y_x) | X'_t = x])^2 \\ &\leq |\mathcal{X}| \sum_{x_1, x_2 \in \mathcal{X}} \tilde{\mathbb{P}}_{t-1}(x_1) \tilde{\mathbb{P}}_{t-1}(x_2) (\mathbb{E}_{t-1}[q_t(x_1, Y_{x_1})] - \mathbb{E}_{t-1}[q_t(x_1, Y_{x_1}) | X'_t = x_2])^2 \\ &\leq \frac{|\mathcal{X}| B^2}{2} \sum_{x_1, x_2 \in \mathcal{X}} \tilde{\mathbb{P}}_{t-1}(x_1) \tilde{\mathbb{P}}_{t-1}(x_2) \text{KL}(\mathbb{P}_{t-1}(Y_{x_1} | X'_t = x_2) \| \mathbb{P}_{t-1}(x_1)) \\ &= \frac{1}{2} |\mathcal{X}| B^2 \mathbb{I}_{t-1}(X'_t; (X_t, Y_{X_t})) \leq \frac{1}{2} |\mathcal{X}| B^2 \mathbb{I}_{t-1}(\theta_*; (X_t, Y_{X_t})) \end{aligned}$$

553 Here, the second step uses the Cauchy-Schwarz inequality and the third step uses the fact that the  
 554 previous line can be viewed as the diagonal terms in a sum over  $x_1, x_2$ . The fourth step uses a version  
 555 of Pinsker's inequality given in Lemma 4 of Appendix A and the fifth step uses the second result of  
 556 Lemma 8. The last step uses Lemma 6 and the fact that  $X'_t$  is a deterministic function of  $\theta_*$  given  
 557  $D_{t-1}$ . Now, using (7) and the Cauchy-Schwarz inequality we have,

$$\mathbb{E}[J(\theta_*, \pi_M^{\text{PS}}) - J(\theta_*, \pi_M^*)]^2 \leq n \sum_{t=1}^n \frac{1}{2} |\mathcal{X}| B^2 \mathbb{I}_{t-1}(\theta_*; (X_t, Y_{X_t})) = \frac{1}{2} |\mathcal{X}| B^2 \mathbb{I}(\theta_*; D_n)$$

Here the last step uses the chain rule of mutual information in the following form,

$$\sum_t I_{t-1}(\theta_*; (X_t, Y_{X_t})) = \sum_t I(\theta_*; (X_t, Y_{X_t}) | \{(X_j, Y_{X_j})\}_{j=1}^{t-1}) = I(\theta_*; \{(X_j, Y_{X_j})\}_{j=1}^n).$$

The claim follows from the observation,  $I(\theta_*; D_n) \leq \Psi_n$ .  $\square$

### B.3 Proof of Theorem 3

Let  $D$  be the data sequence collected by a policy  $\pi$ . For brevity, let  $\bar{\lambda}(D) = \mathbb{E}[\lambda(\theta_*, D)]$  denote the expected penalty when executing policy  $\pi$  for given  $\theta_*$ . Note that  $\bar{\lambda}$  is a function of the policy  $\pi$ . For example, if  $D_1, D_2$  was collected by policies  $\pi_1, \pi_2$ ,  $\bar{\lambda}(D_1 \uplus D_2)$  will denote the expected penalty of the policy which executes  $\pi_1$  for  $|D_1|$  steps, then starts executing  $\pi_2$  without considering the data collected by  $\pi_1$ . We begin with the following Lemma which shows that  $\pi_M^*$  performs as well as the globally optimal adaptive policy  $\pi_G^*$  up to a constant factor. Note that both  $\pi_M^*$  and  $\pi_G^*$  know  $\theta_*$ .

**Lemma 10.** *Let  $D_m^{**}$  be the data collected  $\pi_G^*$  in  $m$  steps and  $D_n^*$  be the data collected by  $\pi_M^*$  in  $n$  steps. Then, under condition 2,*

$$\bar{\lambda}(D_n^*) \leq \bar{\lambda}(D_m^{**}) + e^{-\frac{n}{m}} (1 - \bar{\lambda}(D_m^{**}))$$

*Proof.* The proof follows the analysis of similar greedy algorithms under submodularity assumptions [24, 35]. We begin with the following calculations for  $t < n$ . For  $t \leq n$ , let  $D_t^*$  be the first  $t$  points collected by  $\pi_M^*$ . For  $j \leq m$ , let  $D_j^{**}$  be the first  $j$  points collected by  $\pi_G^*$ , and  $X_j^{**}$  be the  $j^{\text{th}}$  point collected by  $\pi_G^*$ . We have,

$$\begin{aligned} \bar{\lambda}(D_m^{**}) &\geq \bar{\lambda}(D_t^* \uplus D_m^{**}) = \bar{\lambda}(D_t^*) + \sum_{j=1}^m \left( \bar{\lambda}(D_t^* \uplus D_j^{**}) - \bar{\lambda}(D_t^* \uplus D_{j-1}^{**}) \right) \\ &\geq \bar{\lambda}(D_t^*) + \sum_{j=1}^m \left( \bar{\lambda}(D_t^* \uplus \{(X_j^{**}, Y_{X_j^{**}})\}) - \bar{\lambda}(D_t^*) \right) \geq \bar{\lambda}(D_t^*) + \sum_{j=1}^m \left( \bar{\lambda}(D_{t+1}^*) - \bar{\lambda}(D_t^*) \right) \end{aligned} \quad (12)$$

Here, the first step uses monotonicity on  $\lambda$  (condition 2), and the second step is a telescoping sum. The third step uses the diminishing returns property in condition 2 noting that  $D_t^* \uplus D_{j-1}^{**} \supset D_t^*$ ; note that  $X_j^{**}$  is the last element of  $D_j^{**}$ . The last step uses that  $\pi_M^*$  chooses the best next action in expectation, and that it knows  $\theta_*$ , and hence  $\mathbb{E}[\lambda(\theta_*, D_{t+1}^*) | D_t^*] \leq \mathbb{E}[\lambda(\theta_*, D_t^* \cup \{(x, Y_x)\}) | D_t^*]$  for all actions  $x \in \mathcal{X}$ .

Now let  $\delta_t = \bar{\lambda}(D_m^{**}) - \bar{\lambda}(D_t^*)$ . Equation (12) takes the form,  $-\delta_t \geq m(\delta_{t+1} - \delta_t)$  which implies  $\delta_{t+1} \leq (1 - 1/m)\delta_t$ . Applying this recursively to obtain  $\delta_n \leq (1 - 1/m)^n \delta_0 \leq e^{-n/m} \delta_0$  and observing that  $\delta_0 = \lambda(\emptyset) - \lambda(D_m^{**}) \leq 1 - \lambda(D_m^{**})$  yields the result.  $\square$

**Proof of (Theorem 3).** Let  $D_n$  be the data collected by  $\pi_M^{\text{PS}}$ . By monotonicity of  $\bar{\lambda}$ , and the fact that the minimum is smaller than the average we have  $\bar{\lambda}(D_n) \leq \frac{1}{n} \sum_{t=1}^n \bar{\lambda}(D_t)$ . Hence,

$$\begin{aligned} \mathbb{E}[\lambda(\theta_*, D_n)] &\leq \mathbb{E} \left[ \frac{1}{n} \sum_{t=1}^n \bar{\lambda}(D_t^*) \right] + B \sqrt{\frac{|\mathcal{X}| \Psi_n}{2n}} \\ &\leq \mathbb{E} \left[ \bar{\lambda}(D_m^{**}) + \frac{1}{n} \sum_{t=1}^n e^{-t/m} (1 - \bar{\lambda}(D_m^{**})) \right] + B \sqrt{\frac{|\mathcal{X}| \Psi_n}{2n}} \\ &\leq \mathbb{E}[\lambda(\theta_*, D_m^{**})] + (1 - \mathbb{E}[\lambda(\theta_*, D_m^{**})]) \frac{1}{n} \sum_{t=1}^n e^{-t/m} + B \sqrt{\frac{|\mathcal{X}| \Psi_n}{2n}} \\ &\leq \mathbb{E}[\lambda(\theta_*, D_m^{**})] + (1 - \mathbb{E}[\lambda(\theta_*, D_m^{**})]) \frac{(1+m)e^{-1/m}}{n} + B \sqrt{\frac{|\mathcal{X}| \Psi_n}{2n}}. \end{aligned}$$

Here, the first step uses Theorem 2, the second step uses Lemma 10 for each  $t$ . The third step rearranges terms and the last step bounds the sum by an integral to obtain

$$\sum_{t=1}^n e^{-t/m} \leq e^{-1/m} + \int_1^\infty e^{-t/m} dt \leq e^{-1/m} + m e^{-1/m}$$

585 Now, using  $m = \gamma n$  and the fact that  $1 + x \leq e^x$  for  $x > 0$  we have  $(1 + m)e^{-1/m}/n =$   
 586  $\gamma(1 + \frac{1}{\gamma n})e^{-1/(\gamma n)} \leq \gamma$ . The second statement follows from the first statement by substituting  
 587  $\mu = 1 - \lambda$ . □
